# Supplementary material for: ThreeDWorld: A Platform for Interactive Multi-Modal Physical Simulation
Source: arXiv:2007.04954 source file (2021-12-28)
Supplement: Supplementary file 1 [file alter_example_controller.tex]

\subsection{Example Controller}\label{example_controller}

The following controller will create this image:

\includegraphics[width=0.6\linewidth]{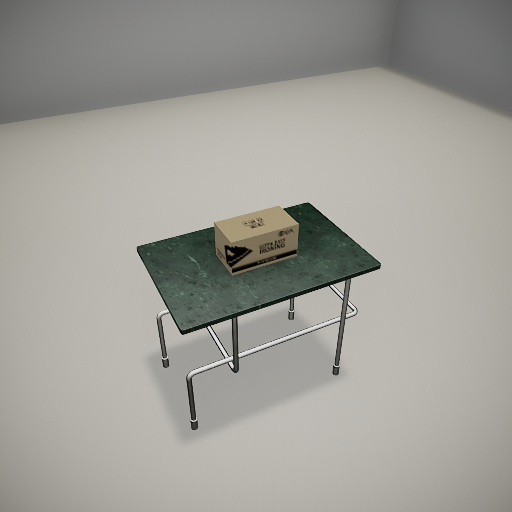}

\begin{verbatim}
from tdw.controller import Controller
from tdw.tdw_utils import TDWUtils
from tdw.output_data import Bounds, OutputData

# Create the controller and create a 12x12 room.
c = Controller()
c.start()
c.communicate(TDWUtils.create_empty_room(12, 12))

# Create the desk.
desk_id = Controller.get_unique_id()
c.communicate({"$type": "add_object",
               "model_name": "small_table_green_marble",
               "id": desk_id})
# Receive the bounds.
resp = c.communicate({"$type": "send_bounds",
                      "frequency": "once",
                      "ids": [desk_id]})
# Get the bounds data of the desk.
top = Bounds(resp[0]).get_top(0)

# Place a box on top of the desk.
box_id = c.get_unique_id()
c.communicate({"$type": "add_object",
               "id": box_id,
               "model_name": "iron_box",
               "position": {"x": 0,
                            "y": top[1],
                            "z": 0}})

avatar_id = "a"
# Create an avatar so that the build will render.
c.communicate({"$type": "create_avatar",
               "type": "A_Img_Caps_Kinematic",
               "id": avatar_id})

# Teleport the avatar and look at the object.
c.communicate([{"$type": "teleport_avatar_to",
                "avatar_id": avatar_id,
                "position": {"x": 1, 
                             "y": 2.5,
                             "z": 2}},
               {"$type": "look_at",
                "avatar_id": avatar_id,
                "object_id": box_id}])
\end{verbatim}
